# Supplementary material for: Certifying Safety in Reinforcement Learning under Adversarial Perturbation Attacks
Source: arXiv:2212.14115 source file (2022-12-28)
Supplement: Supplementary file 1 [file appendix.tex]

\section*{Supplementary Materials}

\section{Results for $l_2$ Norm}
For $l_2$ norm, we perform training with noise added to the image. 
More specifically, for $g(o)$ (mapping visual inputs to state in our experiments), we add noise $\eta \sim \sigma N(0,1)$ to the image, where $\sigma$ is the exogenously specified standard deviation, and push both the clean image and image with noise to the buffer. For adversarial training, every time we sample from the buffer and obtain $(o, a, r, o')$, where $o$ is the current observation and $o'$ is the next observation, we add the noise $\sigma N(0,1)$ to $o$ and then perform training either using IBP (in the case of RADIAL, PSRL-AT, and PSRL-Hybrid), or FGSM with a random start in the case of AT~\citep{wong2020fast}. 

For certifying $g(o)$, we use median smoothing in Lemma \ref{pert_smooth}~\citep{chiang2020detection} to calculate the upper and lower bound for each feature of the predicted state $s$, and then use $\beta$-CROWN for certifying the policy $\pi_s$ (since feature-by-feature median smoothing certificates effectively turn input perturbations to $\pi_s$ into $\ell_\infty$-norm perturbations).
We reproduce the median smoothing lemma here for completeness.
\begin{lemma}[\citet{chiang2020detection}]
\label{pert_smooth}
A percentile-smoothed function $h_p$ with adversarial perturbation $\delta$ can be bounded as
\begin{equation}
    h_{\underline{p}}(x) \leq h_{p}(x+\delta) \leq h_{\bar{p}}(x) \quad \forall\|\delta\|_{2}<\epsilon,
\end{equation}
where $h_p(x) = \{y\in\mathbb{R}|\mathbb{P}[f(x+G)\leq y ] = p\}, G\sim N(0,\sigma^2I)$ (the $p$-th percentile), $\underline{p}:=\Phi\left(\Phi^{-1}(p)-\frac{\epsilon}{\sigma}\right)$ and $\bar{p}:=\Phi\left(\Phi^{-1}(p)+\frac{\epsilon}{\sigma}\right)$, with $\Phi$ being the standard Gaussian CDF.
\end{lemma}

\section{Efficacy of $\ell_2$ Adversarially Trained Models}

Figure~\ref{F:reward-cert_l2} (left) presents nominal reward for both the PSRL (referred to as Vanilla) and the adversarial training methods for the $\ell_2$-norm perturbations.
\begin{figure}[h!]
\centering
\begin{tabular}{c}

\includegraphics[width=0.94\linewidth]{l2norm_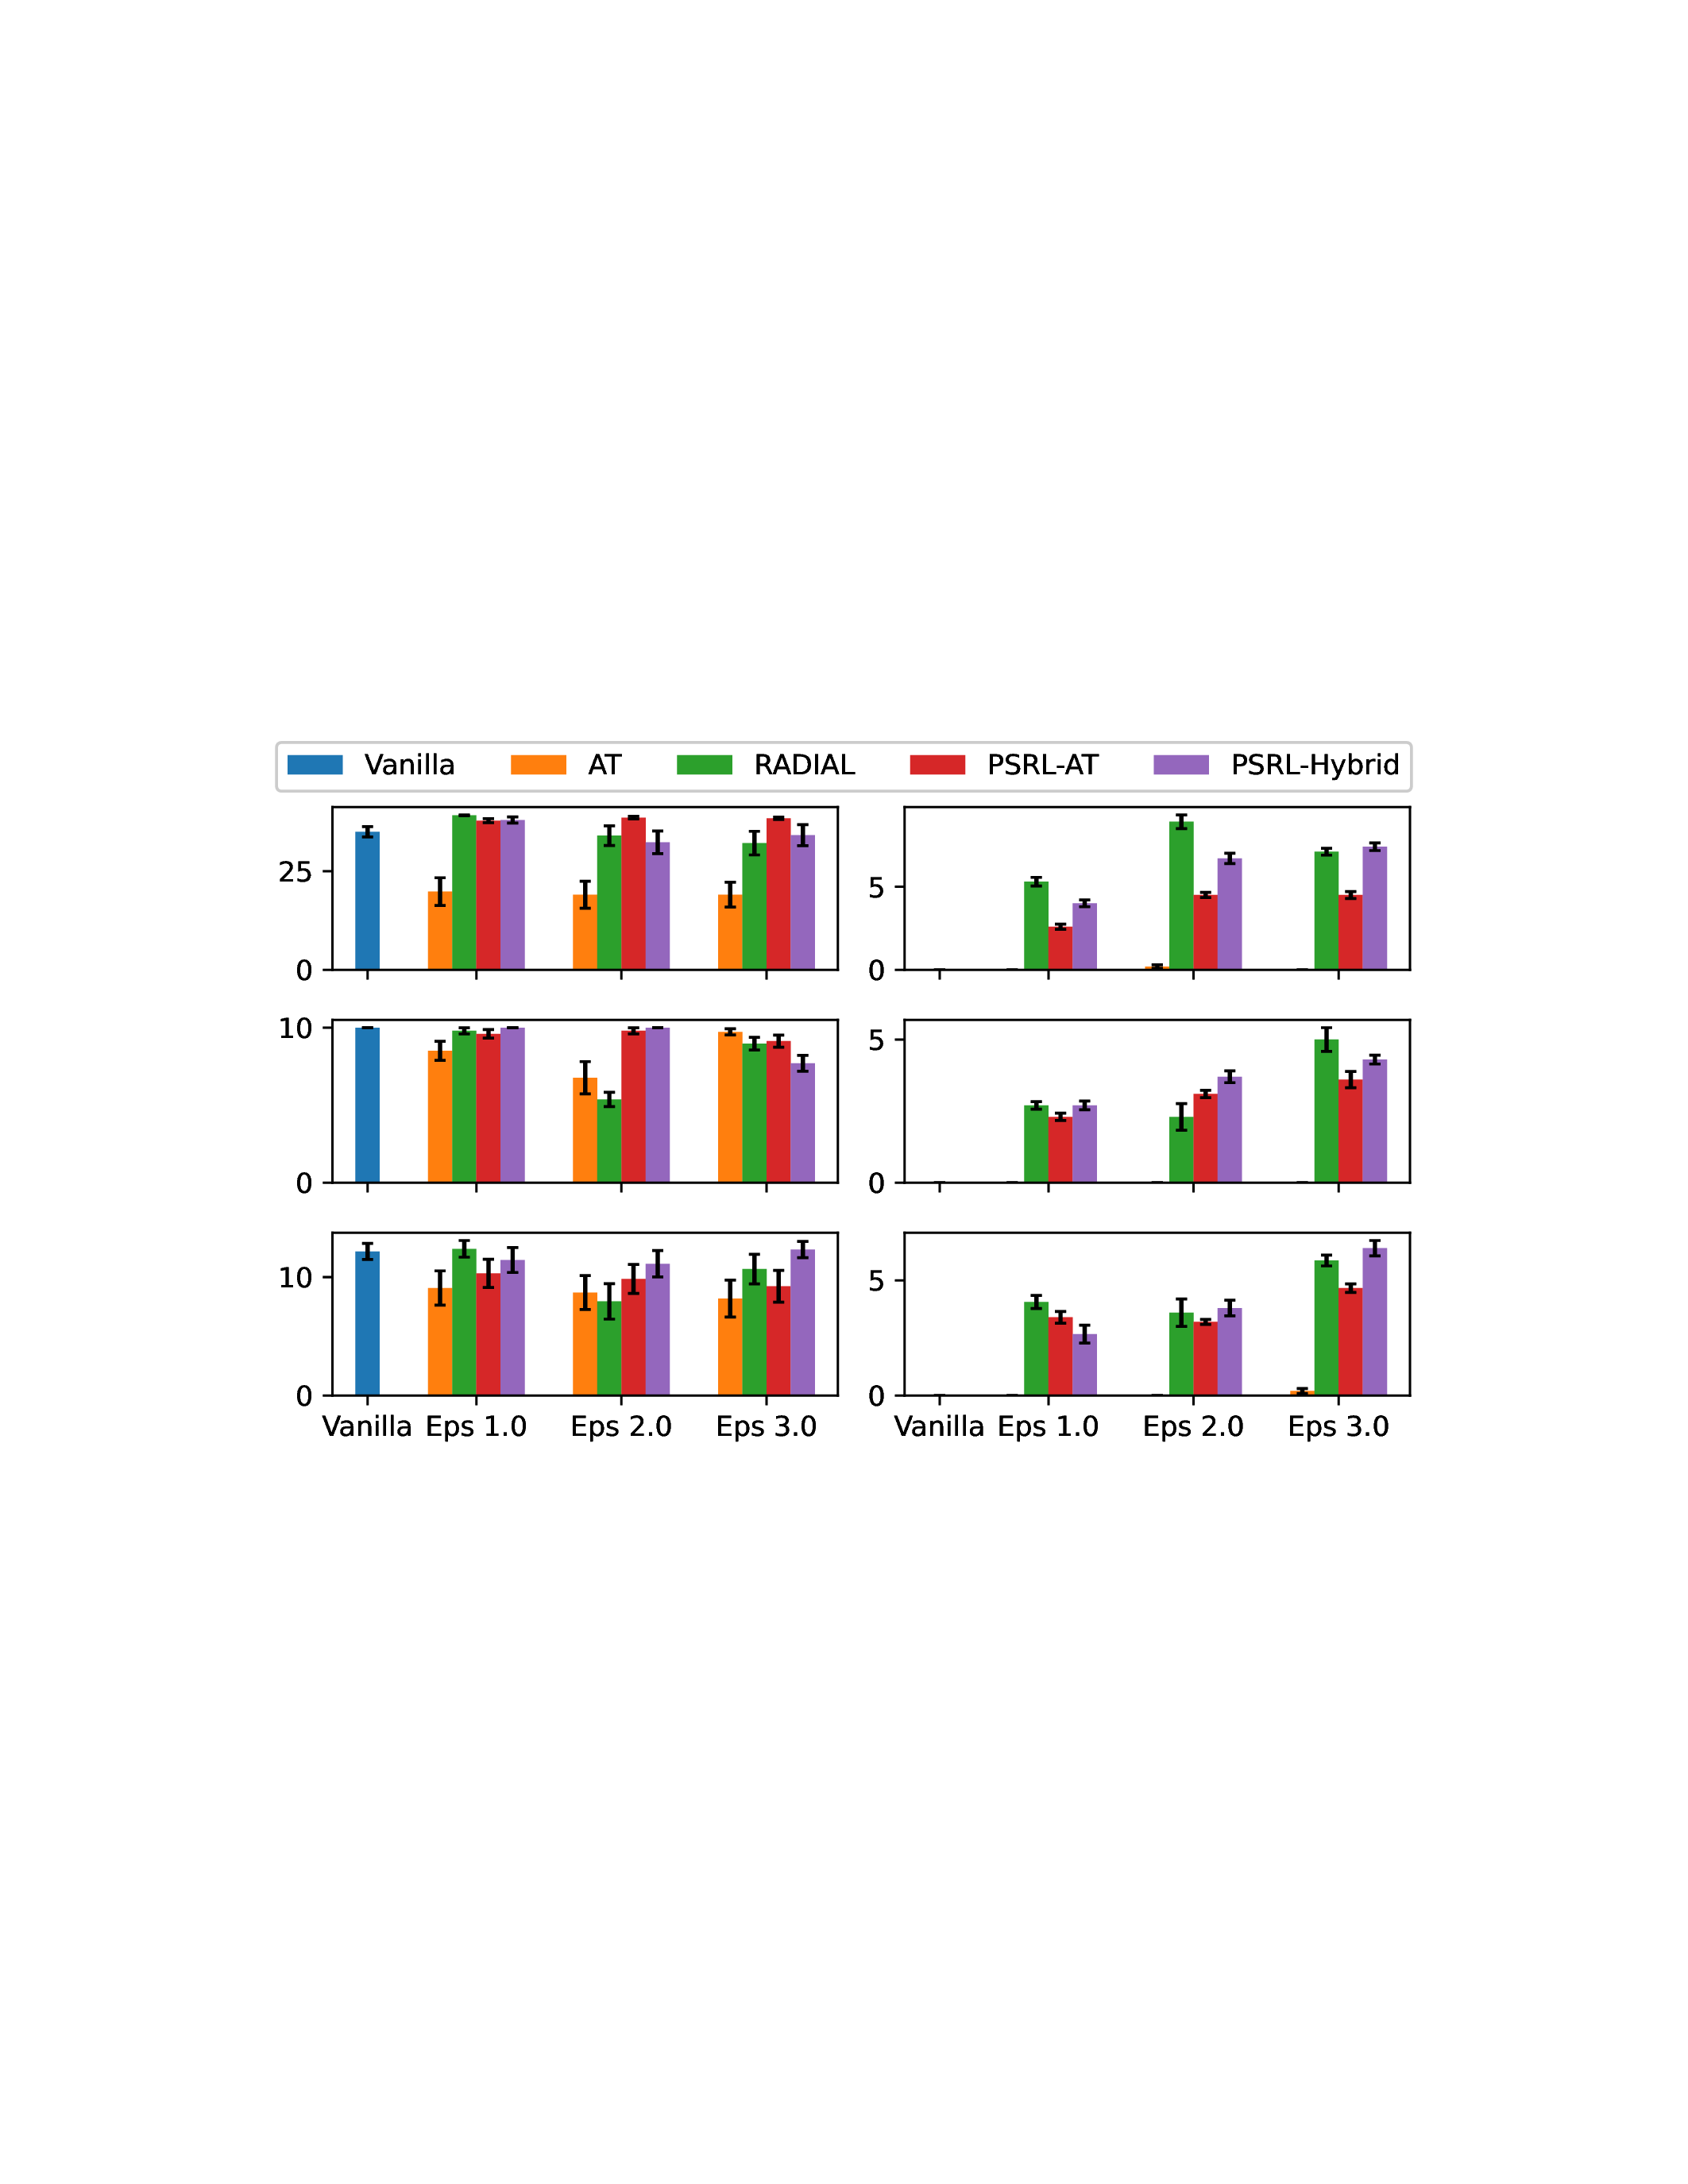}
\end{tabular}
\caption{Averaged reward (left) and certified safety (right) for Highway (top), Twoway (middle) and Exit (bottom) for $l_2$ norm.}
\label{F:reward-cert_l2}
\end{figure}
The results are largely consistent with what we presented in the main paper for $\ell_\infty$-norm perturbations: AT fairs rather poorly, while the remaining three methods typically yield near-optimal reward in most cases, with PSRL-Hybrid typically the best or nearly best of the methods.

Figure~\ref{F:reward-cert_l2} (right) presents adversarial certified safety for $T_v=5$.
Here again we see a similar pattern: AT performs quite poorly, while both PSRL-AT and PSRL-Hybrid generally yield the best certificates, with RADIAL usually, but not always, performing comparably to at least one of these.

\begin{figure}[h!]
\centering
\begin{tabular}{cc}
\includegraphics[width=0.47\linewidth]{l2norm_highway_twoway_exit_far.eps} &
\includegraphics[width=0.47\linewidth]{l2norm_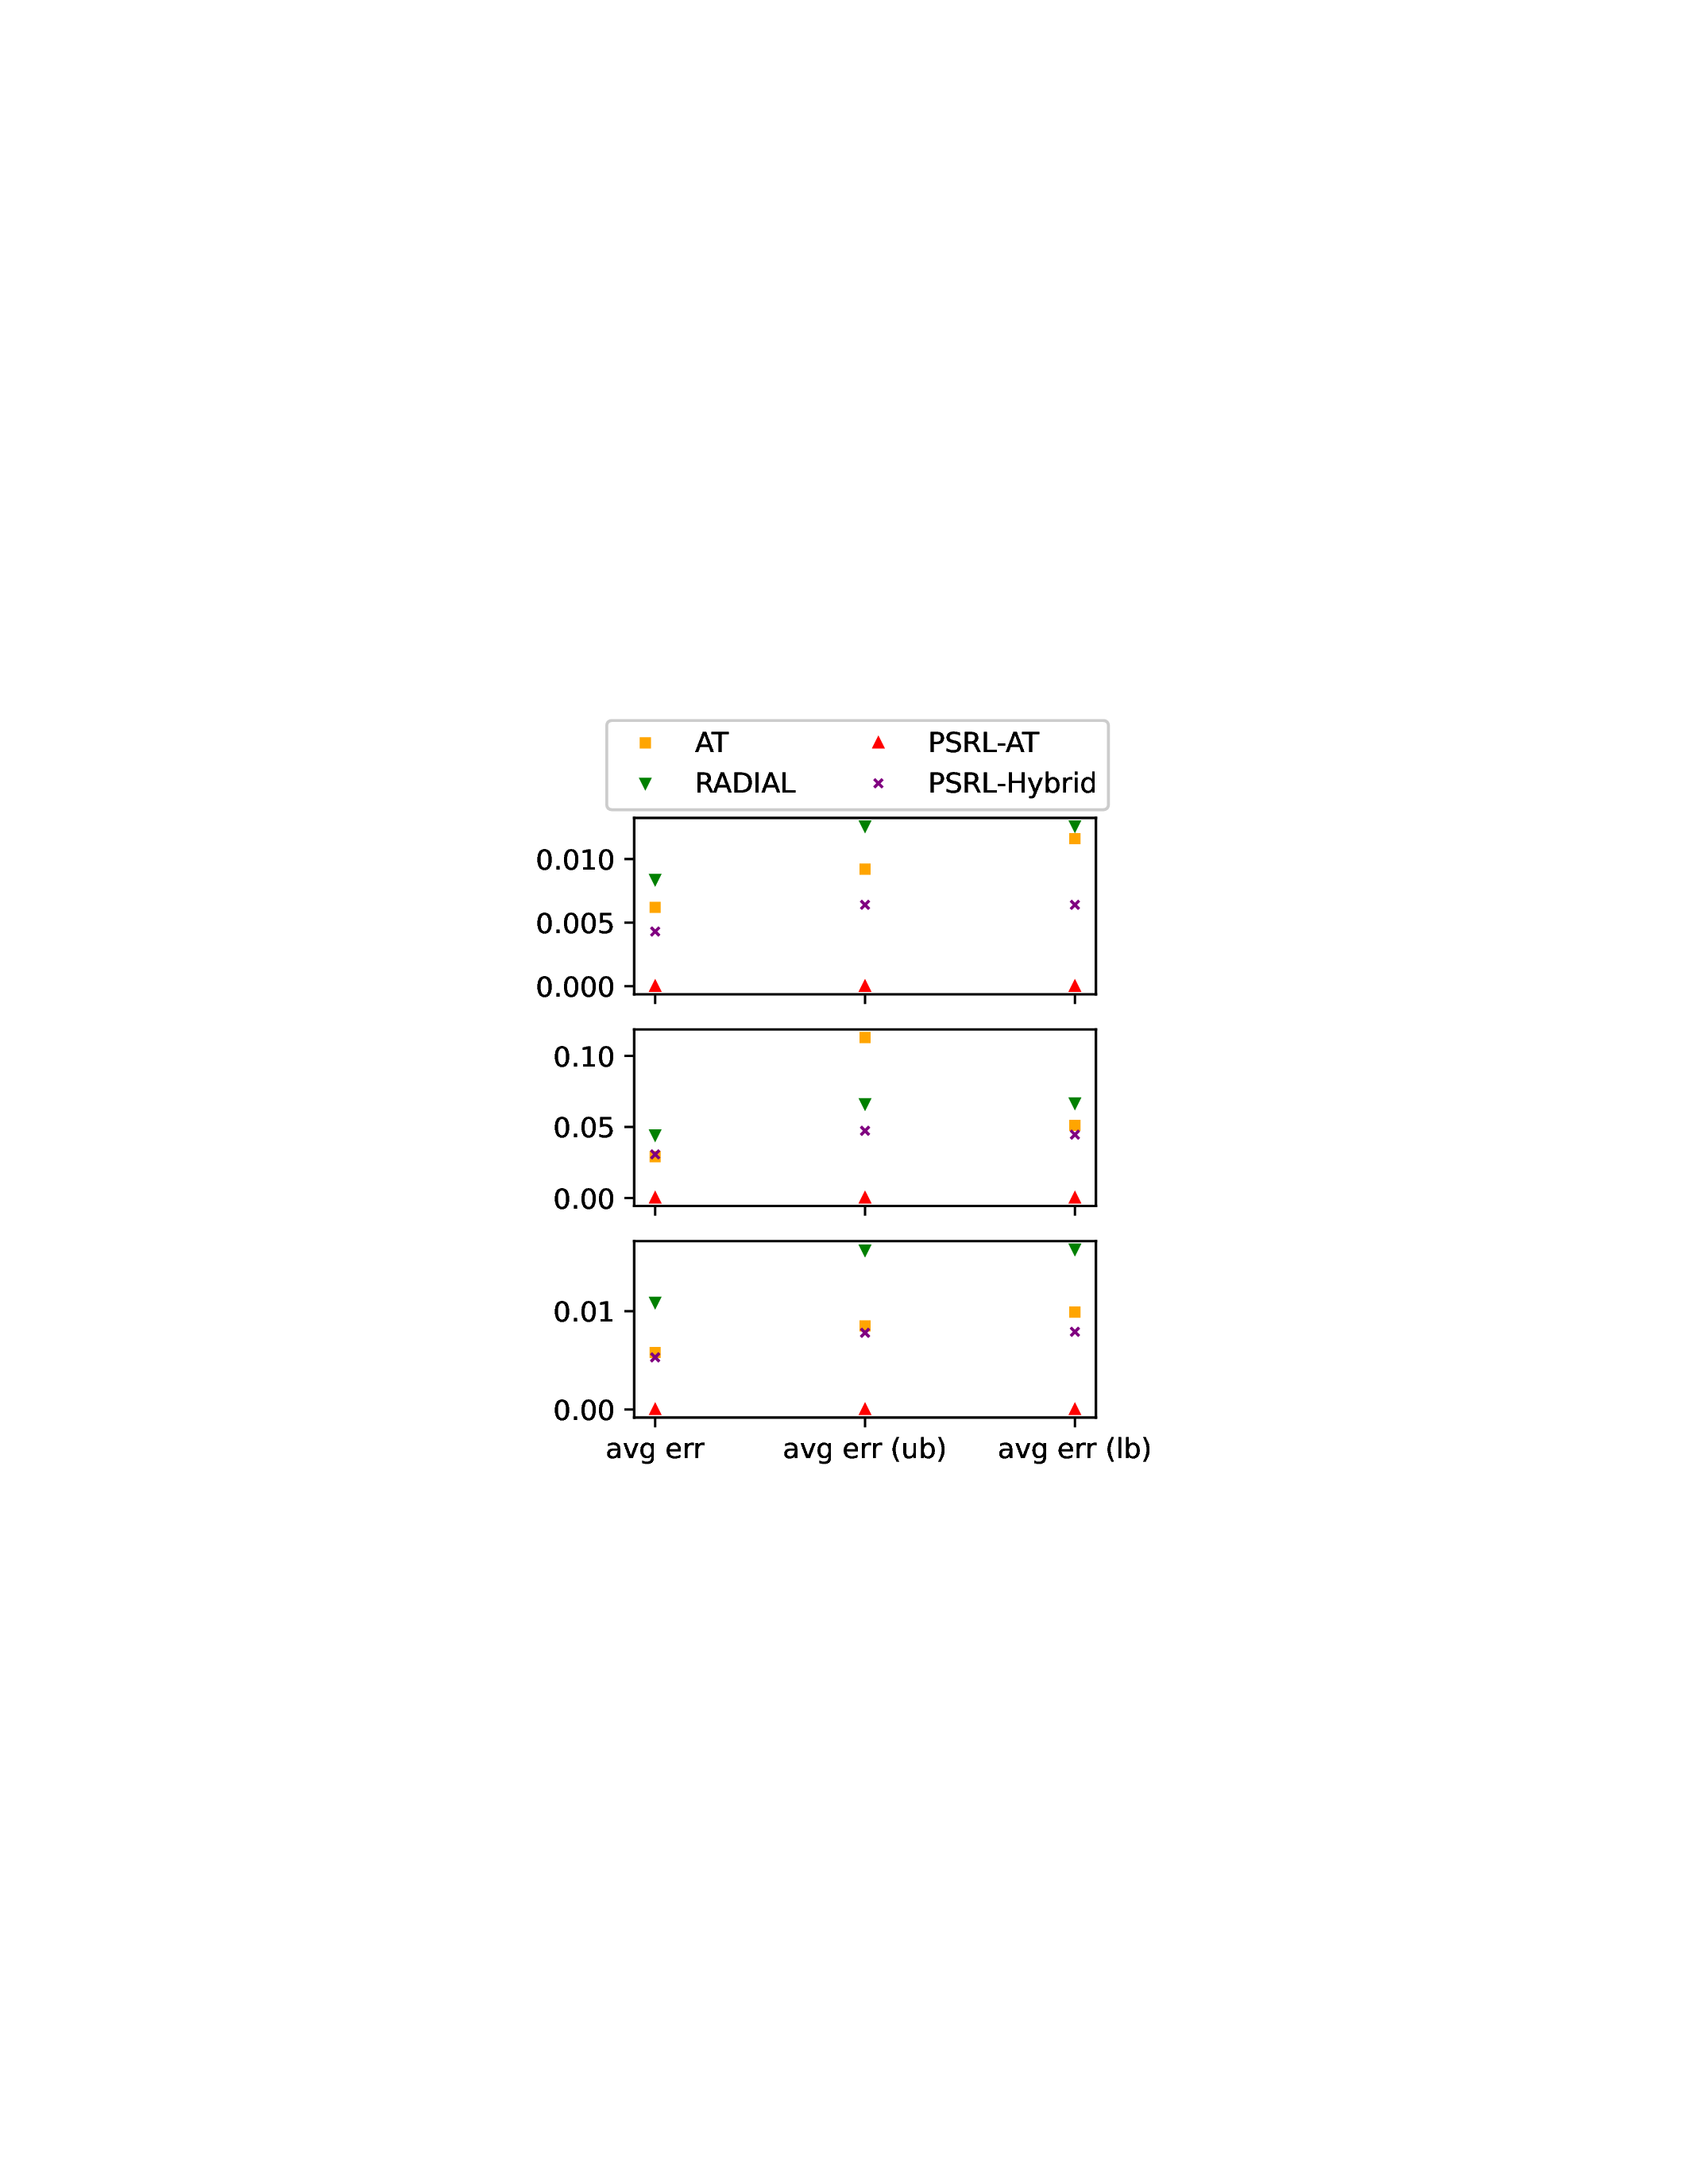}
\end{tabular}
\caption{False action rate (left) and MSE of state prediction error (right) for Twoway (middle) and Exit (bottom)
for $l_2$ norm.}
\label{F:error_l2}
\end{figure}
Figure~\ref{F:error_l2} presents the results for false action rate (left) and MSE (right), and the results again echo what we had observed for $\ell_\infty$ norm, with PSRL-AT typically yielding far better performance in both compared to all others.

\section{Certification Results for 10 and 15 Steps}

The certification results for 10 and 15 steps are shown in Figure \ref{cert_lin2_10_15} ($l_\infty$ norm) and Figure \ref{cert_lin2_10_15} ($l_2$ norm).
Here there is again broad consistency with our earlier discussion, but with several interesting exceptions.
In particular, we see that---particularly for the $\ell_\infty$ norm---RADIAL exhibits high variation in performance, and occasionally rather poor robustness certificates compared to other methods (e.g., for $T_v=15$).
\begin{figure}[h!]
\centering
\begin{tabular}{c}

\includegraphics[width=0.94\linewidth]{l_inf_10_15.eps}
\end{tabular}
\caption{Results for $l_\infty$ norm. 10 steps (left) and 15 steps (right) for Highway (top), Twoway (middle) and Exit (bottom).
}
\label{cert_linf_10_15}
\end{figure}
\begin{figure}[h!]
\centering
\begin{tabular}{c}

\includegraphics[width=0.94\linewidth]{l2norm_10_15_cert.eps}
\end{tabular}
\caption{Results for $l_2$ norm. 10 steps (left) and 15 steps (right) for Highway (top), Twoway (middle) and Exit (bottom).
}
\label{cert_lin2_10_15}
\end{figure}

\section{Efficacy of TASC}
Here we present the total median number of nodes explored. Note that the number of nodes possible is 781 for 5 steps, 2,441,406 for 10 steps and 7,629,394,531 for 15 steps. We cap the total number of nodes allowed to be explored to $M=500$, however, as we presented below, it does not impact our median results for $l_\infty$ norm, and only impact Vanilla and AT result for \textit{Highway} environment under $l_2$ norm. For $l_\infty$ norm, it is presented in Table \ref{l_inf_total_nodes} and for $l_2$ norm it is presented in Table \ref{l_2_total_nodes}. 
\begin{table}[!h]
\centering
\begin{tabular}{cccc}
\hline\hline
\multicolumn{4}{c}{Highway}                                   \\\hline
                & 5 step & 10 step & 15 step \\\hline
\multicolumn{1}{l|}{Vanilla}     & 33     & 12      & 19      \\
\multicolumn{1}{l|}{AT}          & 12     & 10      & 19      \\
\multicolumn{1}{l|}{RADIAL}      & 30     & 116     & 379     \\
\multicolumn{1}{l|}{PSRL-AT}     & 20     & 52      & 174     \\
\multicolumn{1}{l|}{PSRL-Hybrid} & 29     & 154     & 307     \\
\hline\hline
\multicolumn{4}{c}{Twoway}                                    \\\hline
                                 & 5 step & 10 step & 15 step \\\hline
\multicolumn{1}{l|}{Vanilla}     & 5      & 11      & 15      \\
\multicolumn{1}{l|}{AT}          & 5      & 11      & 15      \\
\multicolumn{1}{l|}{RADIAL}      & 9      & 25      & 27      \\
\multicolumn{1}{l|}{PSRL-AT}     & 8      & 47      & 51      \\
\multicolumn{1}{l|}{PSRL-Hybrid} & 13     & 62      & 73      \\
\hline\hline
\multicolumn{4}{c}{Exit}                                      \\\hline
                                 & 5 step & 10 step & 15 step \\\hline
\multicolumn{1}{l|}{Vanilla}     & 5      & 10      & 15      \\
\multicolumn{1}{l|}{AT}          & 8      & 17      & 17      \\
\multicolumn{1}{l|}{RADIAL}      & 6      & 21      & 19      \\
\multicolumn{1}{l|}{PSRL-AT}     & 9      & 13      & 15      \\
\multicolumn{1}{l|}{PSRL-Hybrid} & 7      & 22      & 15     \\\hline
\end{tabular}
\caption{\textsc{TASC}: total number of nodes explored ($l_\infty$ norm).}
\label{l_inf_total_nodes}

\end{table}

\begin{table}[!h]
\centering
\begin{tabular}{cccc}
\hline\hline
\multicolumn{4}{c}{Highway}                                   \\\hline
                                 & 5 step & 10 step & 15 step \\\hline
\multicolumn{1}{l|}{Vanilla}     & 41     & 500     & 500     \\
\multicolumn{1}{l|}{AT}          & 16     & 150     & 500     \\
\multicolumn{1}{l|}{RADIAL}      & 5      & 10      & 20      \\
\multicolumn{1}{l|}{PSRL-AT}     & 5      & 10      & 17      \\
\multicolumn{1}{l|}{PSRL-Hybrid} & 5      & 10      & 20      \\
\hline\hline
\multicolumn{4}{c}{Twoway}                                    \\\hline
                                 & 5 step & 10 step & 15 step \\\hline
\multicolumn{1}{l|}{Vanilla}     & 20     & 63      & 20      \\
\multicolumn{1}{l|}{AT}          & 10     & 44      & 22      \\
\multicolumn{1}{l|}{RADIAL}      & 6      & 13      & 18      \\
\multicolumn{1}{l|}{PSRL-AT}     & 5      & 13      & 15      \\
\multicolumn{1}{l|}{PSRL-Hybrid} & 8      & 15      & 19      \\
\hline\hline
\multicolumn{4}{c}{Exit}                                      \\\hline
                                 & 5 step & 10 step & 15 step \\\hline
\multicolumn{1}{l|}{Vanilla}     & 8      & 13      & 15      \\
\multicolumn{1}{l|}{AT}          & 7      & 14      & 15      \\
\multicolumn{1}{l|}{RADIAL}      & 5      & 10      & 10      \\
\multicolumn{1}{l|}{PSRL-AT}     & 5      & 10      & 11      \\
\multicolumn{1}{l|}{PSRL-Hybrid} & 5      & 10      & 12     \\\hline
\end{tabular}
\caption{\textsc{TASC}: total number of nodes explored ($l_2$ norm).}
\label{l_2_total_nodes}
\end{table}

\section{Environment Setting}
We take two consecutive frames as the image input. The ego vehicle is located at the right side of the image (10\%). See Figure \ref{F:env_img} for demonstration. We take the grayscale image beween the rightmost and left most lanes. Note that the input image for \textit{Exit} environment is similar to Highway, in the figure below we demonstrate the exit lane. The input image for \textit{Highway} and \textit{Exit} is of size $(100, 25)$, and for \textit{Twoway} it is $(150, 17)$. 
\begin{figure}[h!]
\centering
\begin{tabular}{cc}
\includegraphics[width=0.5\linewidth]{highway_env_img.eps}
&
\includegraphics[width=0.5\linewidth]{two_env_img.eps}
\end{tabular}
\begin{tabular}{cc}
\includegraphics[width=0.5\linewidth]{exit_env2.eps}     & \includegraphics[width=0.5\linewidth]{exit_env1.eps} 
\end{tabular}
\caption{Images illustrating the experiment environment.  Highway (top left), Twoway (top right), and Exit (bottom). Ego vehicle is colored as green, and other vehicles are colored are yellow or blue.}
\label{F:env_img}
\end{figure}

\section{Hyperparameters and Experiment Details}
\paragraph{Hyperparameters} Our reinforcement learning model implementation is based on \citet{rl-agents}. To ensure fair comparison, we use the same set of hyperparameters across all experiments and the same neural network architecture  within the same environment (please refer to our attached code for the neural network architecture details). For learning $g(o)$, we use buffer size 10000 and batch size 32, and predict positions of two vehicles closest to the ego vehicle in the scene. In case there are less than two vehicles in the scene, the positions defaults to -1 for \textit{Highway} and \textit{Twoway}, and defaults to 0 for \textit{Exit}. For reinforcement learning, most of the hyperparameters are consistent with the original setting in \citet{rl-agents} under the \textit{Highway} environment. For replay buffer we tested under the \textit{Highway} environment and choose the best among \{5000, 10000, 15000\}. For our final model, we use buffer size 10000, batch size 32 and discount factor 0.8 across all environments and experiments (for both $l_2$ and $l_\infty$ norms). In terms of certification, there is no hyperparameter needed for $l_\infty$ norm, and for $l_2$ norm with median smoothing, we use $N = 2000$ samples with $\sigma = 0.05$, and take the cap of the certified robustness as 20/255. That is, once we certify robustness against 20/255, we do not explore further and the algorithm returns 20/255.

\paragraph{Evaluation Details} For each experiment (Vanilla, AT, RADIAL, PSRL-AT and PSRL-Hybrid) and each environment (\textit{Highway}, \textit{Twoway} and \textit{Exit}), we perform three independent runs. For evaluation, we use five seeds for nominal reward and certification. That means, for nominal and certification we report the mean and SEM (standard error of the mean) across 15 evaluation results for each method under each target training epsilon (\{1.0, 2.0, 3.0\}/255). For the MSE error over states prediction, we further take average over three target training epsilon, meaning that the result is averaged over 45 evaluation runs. The duration of the simulation during evaluation is 40 steps for \textit{Highway}, 20 steps for \textit{Twoway} and 15 steps for \textit{Exit}. 

\paragraph{Computational Cost} The training time for  $g(o)$ and reinforcement learning  varies among different environments, but is in general within 1 hours. The running time for adversarial training is 4 hours for each run on a single GeForce RTX 3090 GPU. The certification time varies based on the total number of nodes explored. The maximum running time for a run is 13 minutes where 500 nodes are explored; the majority of the running time is within 5 minutes.
